# Supplementary material for: Heterarchical Granular Dynamics
Source: arXiv:2501.07867 source file (2025-01-14)
Supplement: Supplementary file 1 [file shivu.tex]

\section{Shivu's diffusion --- just for notes, not for publication}

If instead of the above we use Shivu's new measure of diffusivity,

\begin{equation}
    D \propto \frac{\dot\gamma\bar{s}^2}{\sqrt{\phi_\mathrm{cs} - \phi}},
\end{equation}

\noindent this means that $D=\infty$ for solid packings ($\phi=\phi_\mathrm{cs})$, and imaginary for $\phi > \phi_\mathrm{cs}$. %This removes part of the stability criteria for density. We can do the other part by consider the advection velocity more carefully.
I guess this means that the correlation length scale diverges and all of the material gets moved when sheared. This is kind of the opposite of what we need, where we want to have \textbf{no diffusion} when solid. I guess the difference here is that Shivu's model is strain controlled (i.e.\ we always shear at the same \textbf{rate}), whereas ours is more of a mixed condition, where the rate slows down to zero as the material becomes more solid? This is a bit contrary to our idea of things happening \textbf{faster} when the pressure is higher... I'm very confused!

We can add some kind of scaling for $v_y$ with $\phi$. $v_y$ was postulated under the condition that a particle freefalls into a void, and that the size of the void, or what we will now call the mean free path of motion, $l$, is roughly equal to the particle size in a dense medium. We could look for reasonably physical scaling, or begin by noting that such a scaling has the following three conditions:

\begin{enumerate}
    \item At $\phi=1$, $l=0$
    \item At $\phi = \phi_\mathrm{cs}$, $l=\bar s$
    \item At $\phi=0$, $l=\infty$
\end{enumerate}

One simple relationship that satisfies these properties is

\begin{equation}
    \frac{\phi}{\phi_\mathrm{cs}} = \frac{\bar s}{l}
\end{equation}

or

\begin{equation}
    l = \bar s \frac{\phi_\mathrm{cs}}{\phi}
\end{equation}

With this $l$ we then have that

\begin{equation}
    v_y = \sqrt{gl} = \sqrt{g\bar s \frac{\phi_\mathrm{cs}}{\phi}}
\end{equation}
